# Supplementary material for: Bringing Federated Learning to Space
Source: arXiv:2511.14889 source file (2025-11-18)
Supplement: Supplementary file 1 [file Z_Appendicies.tex]

%%%%%%%%%%%%%%%%%%%%%%%%%%%%%%%%%%%%%%%%%%%%%%%%%%%%%%%%%%%%%%%%%%%%%%%%%%%%%%%%%%%%%%%%%%%%%%%%%
\appendices{}              % note there is no {} to put a title. Each appendix has its own title
%%%%%%%%%%%%%%%%%%%%%%%%%%%%%%%%%%%%%%%%%%%%%%%%%%%%%%%%%%%%%%%%%%%%%%%%%%%%%%%%%%%%%%%%%%%%%%%%%
% For a single appendix, use the \appendix{} keyword and do not use the \section command.

\section{More Information}        % first appendix
%%%%%%%%%%%%%%%%%%%%%%%%%%
This is the first appendix. 

\subsection{Comments}
If you have only one appendix, use the ``appendix'' keyword.

\subsection{More Comments}
Use section and subsection keywords as usual.

\section{Summary of Format Requirements}    % second appendix - added 4/10/2025 to be consistent with word template
%%%%%%%%%%%%%%%%%%%%%%%%%%%%%%
\textit{Paper size: }8.5 x 11 inch

 \textit{Number of pages}: 6–20

 \textit{Margins}\\
\hspace*{2em}Top and bottom: 0.75 inch\\
\hspace*{2em}Left and right: 0.75 inch

 \textit{Columns}\\
\hspace*{2em}Number of columns: 2\\
\hspace*{2em}Space between: 0.25 inch

 \textit{Font}: Times Roman 10 pt regular, unless otherwise noted

 \textit{Text}\\
\hspace*{2em}Line spacing: Single\\ 
\hspace*{2em}Space after paragraph: 10 pt\\ 
\hspace*{2em}Paragraph indent: None \\
\hspace*{2em}Justification: Left \& right\\

 \textit{Title}\\
\hspace*{2em}20 pt bold, upper \& lower case, initial caps on all words \hspace*{3em}except articles, conjunctions and prepositions\\
\hspace*{2em}Centered on the full-page width\\
\hspace*{2em}Maximum length 100 characters\\

 \textit{Author(s)}\\
\hspace*{2em}10 pt bold, upper and lower case\\
\hspace*{2em}Centered on the full-page width\\
\hspace*{2em}Name, affiliation, postal address, phone number, and\\\hspace*{3em}e-mail\\
\hspace*{2em}No degrees or titles, except military rank\\

 \textit{Abstract: }9 pt bold

 \textit{Acronyms}: Define acronyms on first usage

 \textit{Page numbers}: Bottom center of each page, including first page

 \textit{Footnotes}: 8 pt regular

 \textit{Headings}\\
\hspace*{2em}Spacing before major or subheadings: Double space\\
\hspace*{2em}Spacing after major or subheadings: 1.5 space\\
\hspace*{2em}Major headings: 12 pt small caps, bold, centered\\
\hspace*{2em}Subheadings: 10 pt italic, flush left, separate line\\
\hspace*{2em}Subsubheadings: 10 pt italic, run into paragraph with\\ 
\hspace*{3em}em dash\\

 \textit{Headers and Footers}\\
\hspace*{2em}No headers\\
\hspace*{2em}Footers used for page numbers and\\
\hspace*{3em}Copyright notice on page 1\\

 \textit{Equations}\\
\hspace*{2em}Centered in column\\
\hspace*{2em}Equation numbers in parentheses, flush right\\
\hspace*{2em}Include special fonts with the paper.\\

 \textit{Figures and Tables}\\
\hspace*{2em}Captions and titles: 10 pt bold\\
\hspace*{2em}Figure captions: Centered directly below figures\\
\hspace*{2em}Table titles: Centered directly above tables\\
\hspace*{2em}Scanned images: 300 dpi JPEG\\

 \textit{References}\\
\hspace*{2em}List references at end of paper.\\
\hspace*{2em}References numbers: In square brackets [ ]\\

 \textit{Biography}\\
\hspace*{2em}Each author's name in bold italic\\
\hspace*{2em}Brief biography in 10 pt italic\\
\hspace*{2em}Photo of each author\\
